# Supplementary material for: Accurate and Efficient Prediction of Double Excitation Energies Using the Particle-Particle Random Phase Approximation
Source: arXiv:2411.16599 ancillary file (2024-11-25)
Supplement: Supplementary file 1 [file si.pdf]

**Supporting Information:**

**Accurate and Efficient Prediction of Double  
Excitation Energies Using the Particle-Particle  
Random Phase Approximation**

Jincheng Yu,<sup>†</sup> Jiachen Li,<sup>‡</sup> Tianyu Zhu,<sup>‡</sup> and Weitao Yang<sup>\*,†</sup>

<sup>†</sup>*Department of Chemistry, Duke University, Durham, North Carolina 27708, United States*

<sup>‡</sup>*Department of Chemistry, Yale University, New Haven, Connecticut 06520, United States*

E-mail: weitao.yang@duke.edu

# 1 Excitation energies of defects obtained from ppRPA

Table S1: Vertical excitation energies of the  $^1A_1$  state of  $NV^-$  in diamond obtained from ppRPA based on different functionals with supercell models containing 63 and 215 atoms. ppRPA calculations were performed in the active space consisting of 200 occupied orbitals and 200 virtual orbitals. The geometry of the  $^3A_2$  ground state and cc-pVDZ basis set were used. All values are in eV.

|                 | supercell 63 | supercell 215 | extrapolated |
|-----------------|--------------|---------------|--------------|
| PBE             | 1.57         | 1.64          | 1.67         |
| B3LYP           | 1.81         | 1.92          | 1.97         |
| CAM-B3LYP       | 1.90         | 2.03          | 2.09         |
| HSE03           | 1.78         | 1.90          | 1.96         |
| M06             | 1.78         | 1.99          | 2.08         |
| M06-2X          | 1.75         | 1.87          | 1.93         |
| SCAN            | 1.63         | 1.73          | 1.77         |
| TPSSh           | 1.66         | 1.78          | 1.83         |
| $\omega$ B97X-D | 1.82         | 1.98          | 2.05         |

# 2 Double excitation energies of molecules obtained from ppRPA

Table S2: Vertical double excitation energies calculated with ppRPA using the aug-cc-pVQZ basis set<sup>S1,S2</sup> with B3LYP functional. All values are in eV.

| system                | state   | electron transition                | ppRPA contribution | $\Delta E$ |
|-----------------------|---------|------------------------------------|--------------------|------------|
| acrolein              | $^1A'$  | $\pi \rightarrow \pi^*$            | 16 16 26.98%       | 7.943      |
| benzoquinone          | $^1A_g$ | $n, n \rightarrow \pi^* \pi^*$     | 29 29 94.64%       | 5.973      |
| borole                | $^1A_1$ | $\pi \rightarrow \pi^*$            | 18 18 3.19%        | 7.393      |
|                       | $^1A_1$ | $\pi, \pi \rightarrow \pi^* \pi^*$ | 18 18 89.78%       | 4.655      |
| butadiene             | $^1A_g$ | $\pi \rightarrow \pi^*$            | 16 16 30.74%       | 6.484      |
| cyclobutadiene        | $^1A_g$ | $\pi, \pi \rightarrow \pi^* \pi^*$ | 15 15 89.74%       | 4.020      |
| cyclopentadiene       | $^1A_1$ | $\pi \rightarrow \pi^*$            | 19 19 35.65%       | 6.490      |
| cyclopentadienethione | $^1A_1$ | $\pi \rightarrow \pi^*$            | n/a                | n/a        |
| cyclopentadienone     | $^1A_1$ | $\pi \rightarrow \pi^*$            | 22 22 9.24%        | 7.688      |
|                       | $^1A_1$ | $\pi, \pi \rightarrow \pi^* \pi^*$ | 22 22 84.40%       | 5.364      |
| diazete               | $^1A_1$ | $\pi, \pi \rightarrow \pi^* \pi^*$ | 15 15 84.87%       | 6.729      |
| ethylene              | $^1A_g$ | $\pi, \pi \rightarrow \pi^* \pi^*$ | 9 9 64.41%         | 12.607     |
| formaldehyde          | $^1A_1$ | $n, n \rightarrow \pi^* \pi^*$     | 9 9 89.36%         | 10.362     |
| glyoxal               | $^1A_g$ | $n, n \rightarrow \pi^* \pi^*$     | 16 16 90.43%       | 5.808      |
| hexatriene            | $^1A_g$ | $\pi \rightarrow \pi^*$            | 23 23 37.05%       | 5.046      |
| naphthalene           | $^1A_g$ | $\pi \rightarrow \pi^*$            | 35 35 41.15%       | 6.414      |
| nitrosomethan         | $^1A'$  | $n, n \rightarrow \pi^* \pi^*$     | 13 13 94.71%       | 4.238      |
| nitrous acid          | $^1A'$  | $n, n \rightarrow \pi^* \pi^*$     | 13 13 95.56%       | 8.513      |
| nitroxyl              | $^1A'$  | $n, n \rightarrow \pi^* \pi^*$     | 9 9 94.91%         | 4.629      |
| octatetraene          | $^1A_g$ | $\pi \rightarrow \pi^*$            | 30 30 39.82%       | 4.140      |
| oxalyl fluoride       | $^1A_1$ | $n, n \rightarrow \pi^* \pi^*$     | 24 24 85.57%       | 9.551      |
| pyrazine              | $^1A_g$ | $n \rightarrow \pi^*$              | 22 22 6.82%        | 8.665      |
|                       | $^1A_g$ | $n, n \rightarrow \pi^* \pi^*$     | 22 22 88.45%       | 8.602      |
| tetrazine             | $^1A_g$ | $n, n \rightarrow \pi^* \pi^*$     | 22 22 95.49%       | 5.211      |
|                       | $^1B_3$ | $n, n \rightarrow \pi^* \pi^*$     | 23 22 97.98%       | 7.000      |
|                       | $^3B_3$ | $n, n \rightarrow \pi^* \pi^*$     | 23 22 99.06%       | 5.990      |

Table S3: Vertical double excitation energies calculated with ppRPA using the aug-cc-pVQZ basis set<sup>S1,S2</sup> with M06-2X functional. All values are in eV.

| system                | state   | electron transition                | ppRPA contribution | $\Delta E$ |
|-----------------------|---------|------------------------------------|--------------------|------------|
| acrolein              | $^1A'$  | $\pi \rightarrow \pi^*$            | n/a                | n/a        |
| benzoquinone          | $^1A_g$ | $n, n \rightarrow \pi^* \pi^*$     | 29 29 91.65%       | 8.064      |
| borole                | $^1A_1$ | $\pi \rightarrow \pi^*$            | 18 18 1.72%        | 7.358      |
|                       | $^1A_1$ | $\pi, \pi \rightarrow \pi^* \pi^*$ | 18 18 89.56%       | 4.810      |
| butadiene             | $^1A_g$ | $\pi \rightarrow \pi^*$            | 16 16 18.91%       | 6.605      |
| cyclobutadiene        | $^1A_g$ | $\pi, \pi \rightarrow \pi^* \pi^*$ | 15 15 89.55%       | 4.062      |
| cyclopentadiene       | $^1A_1$ | $\pi \rightarrow \pi^*$            | 19 19 26.37%       | 6.651      |
| cyclopentadienethione | $^1A_1$ | $\pi \rightarrow \pi^*$            | 26 26 90.13%       | 4.285      |
| cyclopentadienone     | $^1A_1$ | $\pi \rightarrow \pi^*$            | 22 22 5.24%        | 7.670      |
|                       | $^1A_1$ | $\pi, \pi \rightarrow \pi^* \pi^*$ | 22 22 84.27%       | 5.544      |
| diazete               | $^1A_1$ | $\pi, \pi \rightarrow \pi^* \pi^*$ | n/a                | n/a        |
| ethylene              | $^1A_g$ | $\pi, \pi \rightarrow \pi^* \pi^*$ | 9 9 41.27%         | 13.338     |
| formaldehyde          | $^1A_1$ | $n, n \rightarrow \pi^* \pi^*$     | 9 9 85.90%         | 10.069     |
| glyoxal               | $^1A_g$ | $n, n \rightarrow \pi^* \pi^*$     | 16 16 90.76%       | 6.304      |
| hexatriene            | $^1A_g$ | $\pi \rightarrow \pi^*$            | 23 23 31.60%       | 5.578      |
| naphthalene           | $^1A_g$ | $\pi \rightarrow \pi^*$            | 35 35 38.21%       | 7.060      |
| nitrosomethan         | $^1A'$  | $n, n \rightarrow \pi^* \pi^*$     | 13 13 93.21%       | 4.145      |
| nitrous acid          | $^1A'$  | $n, n \rightarrow \pi^* \pi^*$     | 13 13 93.39%       | 8.624      |
| nitroxyl              | $^1A'$  | $n, n \rightarrow \pi^* \pi^*$     | 9 9 93.33%         | 4.620      |
| octatetraene          | $^1A_g$ | $\pi \rightarrow \pi^*$            | 30 30 36.49%       | 4.767      |
| oxalyl fluoride       | $^1A_1$ | $n, n \rightarrow \pi^* \pi^*$     | 24 24 1.00%        | 9.268      |
| pyrazine              | $^1A_g$ | $n \rightarrow \pi^*$              | 22 22 95.00%       | 8.983      |
|                       | $^1A_g$ | $n, n \rightarrow \pi^* \pi^*$     | n/a                | n/a        |
| tetrazine             | $^1A_g$ | $n, n \rightarrow \pi^* \pi^*$     | 22 22 96.08%       | 5.751      |
|                       | $^1B_3$ | $n, n \rightarrow \pi^* \pi^*$     | 23 22 97.38%       | 7.515      |
|                       | $^3B_3$ | $n, n \rightarrow \pi^* \pi^*$     | 23 22 98.38%       | 6.565      |

Table S4: Vertical double excitation energies calculated with ppRPA using the aug-cc-pVQZ basis set<sup>S1,S2</sup> with TPSSh functional. All values are in eV.

| system                | state   | electron transition                | ppRPA contribution | $\Delta E$ |
|-----------------------|---------|------------------------------------|--------------------|------------|
| acrolein              | $^1A'$  | $\pi \rightarrow \pi^*$            | n/a                | n/a        |
| benzoquinone          | $^1A_g$ | $n, n \rightarrow \pi^* \pi^*$     | 29 29 94.81%       | 5.563      |
| borole                | $^1A_1$ | $\pi \rightarrow \pi^*$            | 18 18 3.29%        | 7.476      |
|                       | $^1A_1$ | $\pi, \pi \rightarrow \pi^* \pi^*$ | 18 18 89.81%       | 4.699      |
| butadiene             | $^1A_g$ | $\pi \rightarrow \pi^*$            | 16 16 33.58%       | 6.503      |
| cyclobutadiene        | $^1A_g$ | $\pi, \pi \rightarrow \pi^* \pi^*$ | 15 15 89.85%       | 4.081      |
| cyclopentadiene       | $^1A_1$ | $\pi \rightarrow \pi^*$            | 19 19 37.16%       | 6.531      |
| cyclopentadienethione | $^1A_1$ | $\pi \rightarrow \pi^*$            | n/a                | n/a        |
| cyclopentadienone     | $^1A_1$ | $\pi \rightarrow \pi^*$            | n/a                | n/a        |
|                       | $^1A_1$ | $\pi, \pi \rightarrow \pi^* \pi^*$ | n/a                | n/a        |
| diazete               | $^1A_1$ | $\pi, \pi \rightarrow \pi^* \pi^*$ | n/a                | n/a        |
| ethylene              | $^1A_g$ | $\pi, \pi \rightarrow \pi^* \pi^*$ | 9 9 65.57%         | 12.853     |
| formaldehyde          | $^1A_1$ | $n, n \rightarrow \pi^* \pi^*$     | 9 9 90.05%         | 10.670     |
| glyoxal               | $^1A_g$ | $n, n \rightarrow \pi^* \pi^*$     | 16 16 90.54%       | 5.586      |
| hexatriene            | $^1A_g$ | $\pi \rightarrow \pi^*$            | 23 23 38.69%       | 4.962      |
| naphthalene           | $^1A_g$ | $\pi \rightarrow \pi^*$            | 35 35 42.11%       | 6.323      |
| nitrosomethan         | $^1A'$  | $n, n \rightarrow \pi^* \pi^*$     | 13 13 95.36%       | 4.285      |
| nitrous acid          | $^1A'$  | $n, n \rightarrow \pi^* \pi^*$     | 13 13 95.07%       | 8.555      |
| nitroxyl              | $^1A'$  | $n, n \rightarrow \pi^* \pi^*$     | 9 9 95.56%         | 4.701      |
| octatetraene          | $^1A_g$ | $\pi \rightarrow \pi^*$            | 30 30 41.15%       | 4.012      |
| oxalyl fluoride       | $^1A_1$ | $n, n \rightarrow \pi^* \pi^*$     | 24 24 90.77%       | 9.368      |
| pyrazine              | $^1A_g$ | $n \rightarrow \pi^*$              | n/a                | n/a        |
|                       | $^1A_g$ | $n, n \rightarrow \pi^* \pi^*$     | 22 22 95.34%       | 8.423      |
| tetrazine             | $^1A_g$ | $n, n \rightarrow \pi^* \pi^*$     | 22 22 95.46%       | 4.975      |
|                       | $^1B_3$ | $n, n \rightarrow \pi^* \pi^*$     | 23 22 98.20%       | 6.784      |
|                       | $^3B_3$ | $n, n \rightarrow \pi^* \pi^*$     | 23 22 99.20%       | 5.751      |

Table S5: Vertical double excitation energies calculated with ppRPA using the aug-cc-pVQZ basis set<sup>S1,S2</sup> with PBE functional. All values are in eV.

| system                | state   | electron transition                | ppRPA contribution | $\Delta E$ |
|-----------------------|---------|------------------------------------|--------------------|------------|
| acrolein              | $^1A'$  | $\pi \rightarrow \pi^*$            | n/a                | n/a        |
| benzoquinone          | $^1A_g$ | $n, n \rightarrow \pi^* \pi^*$     | 29 29 94.60%       | 4.901      |
| borole                | $^1A_1$ | $\pi \rightarrow \pi^*$            | n/a                | n/a        |
|                       | $^1A_1$ | $\pi, \pi \rightarrow \pi^* \pi^*$ | n/a                | n/a        |
| butadiene             | $^1A_g$ | $\pi \rightarrow \pi^*$            | 16 16 36.77%       | 6.161      |
| cyclobutadiene        | $^1A_g$ | $\pi, \pi \rightarrow \pi^* \pi^*$ | 15 15 89.15%       | 3.924      |
| cyclopentadiene       | $^1A_1$ | $\pi \rightarrow \pi^*$            | 19 19 38.26%       | 6.238      |
| cyclopentadienethione | $^1A_1$ | $\pi \rightarrow \pi^*$            | n/a                | n/a        |
| cyclopentadienone     | $^1A_1$ | $\pi \rightarrow \pi^*$            | n/a                | n/a        |
|                       | $^1A_1$ | $\pi, \pi \rightarrow \pi^* \pi^*$ | n/a                | n/a        |
| diazete               | $^1A_1$ | $\pi, \pi \rightarrow \pi^* \pi^*$ | n/a                | n/a        |
| ethylene              | $^1A_g$ | $\pi, \pi \rightarrow \pi^* \pi^*$ | 9 9 68.76%         | 12.884     |
| formaldehyde          | $^1A_1$ | $n, n \rightarrow \pi^* \pi^*$     | 9 9 26.94%         | 10.401     |
| glyoxal               | $^1A_g$ | $n, n \rightarrow \pi^* \pi^*$     | 16 16 89.80%       | 4.981      |
| hexatriene            | $^1A_g$ | $\pi \rightarrow \pi^*$            | 23 23 39.89%       | 4.545      |
| naphthalene           | $^1A_g$ | $\pi \rightarrow \pi^*$            | 35 35 42.29%       | 7.406      |
| nitrosomethan         | $^1A'$  | $n, n \rightarrow \pi^* \pi^*$     | 13 13 95.58%       | 4.404      |
| nitrous acid          | $^1A'$  | $n, n \rightarrow \pi^* \pi^*$     | 13 13 1.78%        | 8.240      |
| nitroxyl              | $^1A'$  | $n, n \rightarrow \pi^* \pi^*$     | 9 9 95.89%         | 4.566      |
| octatetraene          | $^1A_g$ | $\pi \rightarrow \pi^*$            | 30 30 41.91%       | 3.594      |
| oxalyl fluoride       | $^1A_1$ | $n, n \rightarrow \pi^* \pi^*$     | 24 24 90.61%       | 8.933      |
| pyrazine              | $^1A_g$ | $n \rightarrow \pi^*$              | n/a                | n/a        |
|                       | $^1A_g$ | $n, n \rightarrow \pi^* \pi^*$     | n/a                | n/a        |
| tetrazine             | $^1A_g$ | $n, n \rightarrow \pi^* \pi^*$     | 22 22 94.32%       | 4.462      |
|                       | $^1B_3$ | $n, n \rightarrow \pi^* \pi^*$     | 23 22 98.23%       | 6.148      |
|                       | $^3B_3$ | $n, n \rightarrow \pi^* \pi^*$     | 23 22 99.27%       | 5.083      |

Table S6: Vertical double excitation energies calculated with ppRPA using the aug-cc-pVQZ basis set<sup>S1,S2</sup> with SCAN functional. All values are in eV.

| system                | state   | electron transition                | ppRPA contribution | $\Delta E$ |
|-----------------------|---------|------------------------------------|--------------------|------------|
| acrolein              | $^1A'$  | $\pi \rightarrow \pi^*$            | n/a                | n/a        |
| benzoquinone          | $^1A_g$ | $n, n \rightarrow \pi^* \pi^*$     | 29 29 95.10%       | 5.465      |
| borole                | $^1A_1$ | $\pi \rightarrow \pi^*$            | 18 18 3.28%        | 7.637      |
|                       | $^1A_1$ | $\pi, \pi \rightarrow \pi^* \pi^*$ | 18 18 90.29%       | 4.758      |
| butadiene             | $^1A_g$ | $\pi \rightarrow \pi^*$            | 16 16 36.70%       | 6.599      |
| cyclobutadiene        | $^1A_g$ | $\pi, \pi \rightarrow \pi^* \pi^*$ | 15 15 90.29%       | 4.158      |
| cyclopentadiene       | $^1A_1$ | $\pi \rightarrow \pi^*$            | 19 19 38.46%       | 6.665      |
| cyclopentadienethione | $^1A_1$ | $\pi \rightarrow \pi^*$            | n/a                | n/a        |
| cyclopentadienone     | $^1A_1$ | $\pi \rightarrow \pi^*$            | n/a                | n/a        |
|                       | $^1A_1$ | $\pi, \pi \rightarrow \pi^* \pi^*$ | n/a                | n/a        |
| diazete               | $^1A_1$ | $\pi, \pi \rightarrow \pi^* \pi^*$ | n/a                | n/a        |
| ethylene              | $^1A_g$ | $\pi, \pi \rightarrow \pi^* \pi^*$ | 9 9 73.14%         | 13.391     |
| formaldehyde          | $^1A_1$ | $n, n \rightarrow \pi^* \pi^*$     | 9 9 91.81%         | 10.816     |
| glyoxal               | $^1A_g$ | $n, n \rightarrow \pi^* \pi^*$     | 16 16 90.94%       | 5.628      |
| hexatriene            | $^1A_g$ | $\pi \rightarrow \pi^*$            | 23 23 40.46%       | 4.921      |
| naphthalene           | $^1A_g$ | $\pi \rightarrow \pi^*$            | 35 35 42.89%       | 6.282      |
| nitrosomethan         | $^1A'$  | $n, n \rightarrow \pi^* \pi^*$     | 13 13 96.34%       | 4.442      |
| nitrous acid          | $^1A'$  | $n, n \rightarrow \pi^* \pi^*$     | 13 13 97.08%       | 8.664      |
| nitroxyl              | $^1A'$  | $n, n \rightarrow \pi^* \pi^*$     | 9 9 96.81%         | 4.748      |
| octatetraene          | $^1A_g$ | $\pi \rightarrow \pi^*$            | 30 30 42.44%       | 3.907      |
| oxalyl fluoride       | $^1A_1$ | $n, n \rightarrow \pi^* \pi^*$     | 24 24 91.71%       | 9.602      |
| pyrazine              | $^1A_g$ | $n \rightarrow \pi^*$              | n/a                | n/a        |
|                       | $^1A_g$ | $n, n \rightarrow \pi^* \pi^*$     | n/a                | n/a        |
| tetrazine             | $^1A_g$ | $n, n \rightarrow \pi^* \pi^*$     | 22 22 95.74%       | 4.866      |
|                       | $^1B_3$ | $n, n \rightarrow \pi^* \pi^*$     | 23 22 98.53%       | 6.752      |
|                       | $^3B_3$ | $n, n \rightarrow \pi^* \pi^*$     | 23 22 99.40%       | 5.704      |

Table S7: Vertical double excitation energies calculated with ppRPA using the aug-cc-pVQZ basis set<sup>S1,S2</sup> with CAM-B3LYP functional. All values are in eV.

| system                | state   | electron transition                | ppRPA contribution | $\Delta E$ |
|-----------------------|---------|------------------------------------|--------------------|------------|
| acrolein              | $^1A'$  | $\pi \rightarrow \pi^*$            | 16 16 19.17%       | 8.157      |
| benzoquinone          | $^1A_g$ | $n, n \rightarrow \pi^* \pi^*$     | n/a                | n/a        |
| borole                | $^1A_1$ | $\pi \rightarrow \pi^*$            | 18 18 2.50%        | 7.454      |
|                       | $^1A_1$ | $\pi, \pi \rightarrow \pi^* \pi^*$ | 18 18 89.87%       | 4.786      |
| butadiene             | $^1A_g$ | $\pi \rightarrow \pi^*$            | 16 16 21.72%       | 6.700      |
| cyclobutadiene        | $^1A_g$ | $\pi, \pi \rightarrow \pi^* \pi^*$ | 15 15 89.62%       | 4.059      |
| cyclopentadiene       | $^1A_1$ | $\pi \rightarrow \pi^*$            | 19 19 30.46%       | 6.650      |
| cyclopentadienethione | $^1A_1$ | $\pi \rightarrow \pi^*$            | 26 26 89.96%       | 4.309      |
| cyclopentadienone     | $^1A_1$ | $\pi \rightarrow \pi^*$            | 22 22 7.45%        | 7.750      |
|                       | $^1A_1$ | $\pi, \pi \rightarrow \pi^* \pi^*$ | 22 22 84.66%       | 5.488      |
| diazete               | $^1A_1$ | $\pi, \pi \rightarrow \pi^* \pi^*$ | 15 15 85.85%       | 6.752      |
| ethylene              | $^1A_g$ | $\pi, \pi \rightarrow \pi^* \pi^*$ | 9 9 52.38%         | 12.240     |
| formaldehyde          | $^1A_1$ | $n, n \rightarrow \pi^* \pi^*$     | 9 9 87.23%         | 10.237     |
| glyoxal               | $^1A_g$ | $n, n \rightarrow \pi^* \pi^*$     | 16 16 90.52%       | 6.371      |
| hexatriene            | $^1A_g$ | $\pi \rightarrow \pi^*$            | 23 23 32.18%       | 5.559      |
| naphthalene           | $^1A_g$ | $\pi \rightarrow \pi^*$            | 35 35 38.54%       | 6.998      |
| nitrosomethan         | $^1A'$  | $n, n \rightarrow \pi^* \pi^*$     | 13 13 93.63%       | 4.192      |
| nitrous acid          | $^1A'$  | $n, n \rightarrow \pi^* \pi^*$     | 13 13 94.57%       | 8.611      |
| nitroxyl              | $^1A'$  | $n, n \rightarrow \pi^* \pi^*$     | 9 9 93.80%         | 4.631      |
| octatetraene          | $^1A_g$ | $\pi \rightarrow \pi^*$            | 30 30 36.00%       | 4.744      |
| oxalyl fluoride       | $^1A_1$ | $n, n \rightarrow \pi^* \pi^*$     | 24 24 1.11%        | 9.486      |
| pyrazine              | $^1A_g$ | $n \rightarrow \pi^*$              | 22 22 93.74%       | 9.052      |
|                       | $^1A_g$ | $n, n \rightarrow \pi^* \pi^*$     | 22 22 1.60%        | 8.846      |
| tetrazine             | $^1A_g$ | $n, n \rightarrow \pi^* \pi^*$     | 22 22 95.86%       | 5.687      |
|                       | $^1B_3$ | $n, n \rightarrow \pi^* \pi^*$     | 23 22 97.60%       | 7.509      |
|                       | $^3B_3$ | $n, n \rightarrow \pi^* \pi^*$     | 23 22 98.71%       | 6.536      |



Table S8: Vertical double excitation energies calculated with ppRPA using the aug-cc-pVQZ basis set<sup>S1,S2</sup> with HSE03 functional. All values are in eV.

| system                | state   | electron transition                | ppRPA contribution | $\Delta E$ |
|-----------------------|---------|------------------------------------|--------------------|------------|
| acrolein              | $^1A'$  | $\pi \rightarrow \pi^*$            | n/a                | n/a        |
| benzoquinone          | $^1A_g$ | $n, n \rightarrow \pi^* \pi^*$     | 29 29 94.82%       | 6.097      |
| borole                | $^1A_1$ | $\pi \rightarrow \pi^*$            | 18 18 3.25%        | 7.563      |
|                       | $^1A_1$ | $\pi, \pi \rightarrow \pi^* \pi^*$ | 18 18 90.00%       | 4.765      |
| butadiene             | $^1A_g$ | $\pi \rightarrow \pi^*$            | 16 16 31.54%       | 6.630      |
| cyclobutadiene        | $^1A_g$ | $\pi, \pi \rightarrow \pi^* \pi^*$ | 15 15 90.16%       | 4.097      |
| cyclopentadiene       | $^1A_1$ | $\pi \rightarrow \pi^*$            | 19 19 36.05%       | 6.627      |
| cyclopentadienethione | $^1A_1$ | $\pi \rightarrow \pi^*$            | n/a                | n/a        |
| cyclopentadienone     | $^1A_1$ | $\pi \rightarrow \pi^*$            | n/a                | n/a        |
|                       | $^1A_1$ | $\pi, \pi \rightarrow \pi^* \pi^*$ | n/a                | n/a        |
| diazete               | $^1A_1$ | $\pi, \pi \rightarrow \pi^* \pi^*$ | 15 15 85.55%       | 6.869      |
| ethylene              | $^1A_g$ | $\pi, \pi \rightarrow \pi^* \pi^*$ | 9 9 66.18%         | 12.764     |
| formaldehyde          | $^1A_1$ | $n, n \rightarrow \pi^* \pi^*$     | 9 9 89.64%         | 10.490     |
| glyoxal               | $^1A_g$ | $n, n \rightarrow \pi^* \pi^*$     | 16 16 90.74%       | 5.946      |
| hexatriene            | $^1A_g$ | $\pi \rightarrow \pi^*$            | 23 23 37.68%       | 5.169      |
| naphthalene           | $^1A_g$ | $\pi \rightarrow \pi^*$            | 35 35 41.53%       | 6.573      |
| nitrosomethan         | $^1A'$  | $n, n \rightarrow \pi^* \pi^*$     | 13 13 94.97%       | 4.291      |
| nitrous acid          | $^1A'$  | $n, n \rightarrow \pi^* \pi^*$     | 13 13 95.28%       | 8.615      |
| nitroxyl              | $^1A'$  | $n, n \rightarrow \pi^* \pi^*$     | 9 9 95.28%         | 4.692      |
| octatetraene          | $^1A_g$ | $\pi \rightarrow \pi^*$            | 30 30 40.59%       | 4.235      |
| oxalyl fluoride       | $^1A_1$ | $n, n \rightarrow \pi^* \pi^*$     | 24 24 89.22%       | 9.783      |
| pyrazine              | $^1A_g$ | $n \rightarrow \pi^*$              | 22 22 95.47%       | 8.737      |
|                       | $^1A_g$ | $n, n \rightarrow \pi^* \pi^*$     | n/a                | n/a        |
| tetrazine             | $^1A_g$ | $n, n \rightarrow \pi^* \pi^*$     | 22 22 95.88%       | 5.327      |
|                       | $^1B_3$ | $n, n \rightarrow \pi^* \pi^*$     | 23 22 98.14%       | 7.150      |
|                       | $^3B_3$ | $n, n \rightarrow \pi^* \pi^*$     | 23 22 99.14%       | 6.146      |

Table S9: Vertical double excitation energies calculated with ppRPA using the aug-cc-pVQZ basis set<sup>S1,S2</sup> with  $\omega$ B97X-D functional. All values are in eV.

| system                | state   | electron transition                | ppRPA contribution | $\Delta E$ |
|-----------------------|---------|------------------------------------|--------------------|------------|
| acrolein              | $^1A'$  | $\pi \rightarrow \pi^*$            | 16 16 21.02%       | 8.181      |
| benzoquinone          | $^1A_g$ | $n, n \rightarrow \pi^* \pi^*$     | n/a                | n/a        |
| borole                | $^1A_1$ | $\pi \rightarrow \pi^*$            | 18 18 2.06%        | 7.606      |
|                       | $^1A_1$ | $\pi, \pi \rightarrow \pi^* \pi^*$ | 18 18 89.55%       | 4.864      |
| butadiene             | $^1A_g$ | $\pi \rightarrow \pi^*$            | 16 16 22.91%       | 6.745      |
| cyclobutadiene        | $^1A_g$ | $\pi, \pi \rightarrow \pi^* \pi^*$ | 15 15 89.61%       | 4.114      |
| cyclopentadiene       | $^1A_1$ | $\pi \rightarrow \pi^*$            | 19 19 31.81%       | 6.671      |
| cyclopentadienethione | $^1A_1$ | $\pi \rightarrow \pi^*$            | 26 26 90.11%       | 4.203      |
| cyclopentadienone     | $^1A_1$ | $\pi \rightarrow \pi^*$            | 22 22 4.61%        | 7.762      |
|                       | $^1A_1$ | $\pi, \pi \rightarrow \pi^* \pi^*$ | 22 22 85.18%       | 5.438      |
| diazete               | $^1A_1$ | $\pi, \pi \rightarrow \pi^* \pi^*$ | 15 15 85.60%       | 6.893      |
| ethylene              | $^1A_g$ | $\pi, \pi \rightarrow \pi^* \pi^*$ | 9 9 11.72%         | 12.456     |
| formaldehyde          | $^1A_1$ | $n, n \rightarrow \pi^* \pi^*$     | 9 9 87.01%         | 10.505     |
| glyoxal               | $^1A_g$ | $n, n \rightarrow \pi^* \pi^*$     | 16 16 90.47%       | 6.251      |
| hexatriene            | $^1A_g$ | $\pi \rightarrow \pi^*$            | 23 23 32.29%       | 5.604      |
| naphthalene           | $^1A_g$ | $\pi \rightarrow \pi^*$            | 35 35 39.01%       | 6.995      |
| nitrosomethan         | $^1A'$  | $n, n \rightarrow \pi^* \pi^*$     | 13 13 94.15%       | 4.230      |
| nitrous acid          | $^1A'$  | $n, n \rightarrow \pi^* \pi^*$     | 13 13 95.24%       | 8.656      |
| nitroxyl              | $^1A'$  | $n, n \rightarrow \pi^* \pi^*$     | 9 9 94.51%         | 4.724      |
| octatetraene          | $^1A_g$ | $\pi \rightarrow \pi^*$            | 30 30 35.55%       | 4.811      |
| oxalyl fluoride       | $^1A_1$ | $n, n \rightarrow \pi^* \pi^*$     | 24 24 2.95%        | 9.745      |
| pyrazine              | $^1A_g$ | $n \rightarrow \pi^*$              | 22 22 94.74%       | 9.014      |
|                       | $^1A_g$ | $n, n \rightarrow \pi^* \pi^*$     | n/a                | n/a        |
| tetrazine             | $^1A_g$ | $n, n \rightarrow \pi^* \pi^*$     | 22 22 95.82%       | 5.614      |
|                       | $^1B_3$ | $n, n \rightarrow \pi^* \pi^*$     | 23 22 97.89%       | 7.427      |
|                       | $^3B_3$ | $n, n \rightarrow \pi^* \pi^*$     | 23 22 98.90%       | 6.441      |

## References

- (S1) Kendall, R. A.; Dunning, T. H.; Harrison, R. J. Electron affinities of the first-row atoms revisited. Systematic basis sets and wave functions. *J. Chem. Phys.* **1992**, *96*, 6796–6806.
- (S2) Woon, D. E.; Dunning Jr, T. H. Gaussian basis sets for use in correlated molecular calculations. III. The atoms aluminum through argon. *J. Chem. Phys.* **1993**, *98*, 1358–1371.
